# Supplementary material for: Reasoning over Multi-view Knowledge Graphs
Source: arXiv:2209.13702 source file (2022-09-27)
Supplement: Supplementary file 1 [file appendix.tex]

\appendix
